# Supplementary material for: Triangular Character Animation Sampling with Motion, Emotion, and Relation
Source: arXiv:2203.04930 source file (2022-03-09)
Supplement: Supplementary file 1 [file _appendix.tex]

\section{Eigenface analysis}
Figure \ref{figure:pca_and_faces} plots the visualization of the eigenfaces corresponding to the top six principal components that explain $78.2\%$ of the total variance. 
\begin{align*}
    \underbrace{f_1, f_2, ...,f_{21}}_{\text{basic faces}}, \xrightarrow{\text{PCA}} eigenfaces \\
    (v,a,d) \xrightarrow{\text{regression}} eigenfaces
\end{align*}
Then we perform a linear regression from VAD scores to the eigenfaces
\begin{figure}[h]
    \centering
    \includegraphics[width=0.95\linewidth]{images/pca_and_faces.pdf}
    \caption{Eigenfaces and the ratio of the variances explained by the number of principal components.}
    \label{figure:pca_and_faces}
\end{figure}

\section{Relation identification}
We compare our method (ST-AOG + MCMC) with other methods to predict the social relations between characters in our good-quality animated scenes. The input features include the one-hot encoding of the labeled names of motions and emotions and VADI scores of motions and emotions obtained from the previous steps. Through those encoding, we run the logistic regression and a two-layer neural network as baselines. We report the performances in Table \ref{table:relation_prediction}. The results demonstrate that our method performs well as the baselines in predicting the types of dominance and intimacy.

\begin{table}[h]
\begin{tabular}{c||cc}
\hline
                             & \textbf{Dominance} & \textbf{Intimacy} \\ \hline \hline
\textbf{Logistic regression} & 43.6\%             & 55.6\%            \\
\textbf{Neural network}      & 44.3\%             & 66.9\%            \\
\textbf{Ours}          & 43.5\%             & 71.4\%            \\ \hline
\end{tabular}
\caption{The training accuracy for different methods. Each method predicts the dominance and intimacy separately as multi-class classification problems.}
\label{table:relation_prediction}
\end{table}

\section{Exploratory analysis of our dataset}

\begin{figure}[h]
    \centering
    \includegraphics[width=0.95\linewidth]{images/label_motion_vadi.pdf}
    \caption{(a) The density plot for the valence and arousal scores of labeled motions. (b) The density plot for the valence and arousal scores of labeled emotions. (Notice that motions and emotions also have dominance scores, but we only show valence and arousal scores for better visualization.) (c) The distribution of the dominance and intimacy scores of labeled relations.}
    \label{figure:label_motion_vadi}
\end{figure}

Figure \ref{figure:label_motion_vadi} plots the distribution of labeled samples' arousal and valence scores of motions and emotions:  a large part of the valence-arousal space is covered. While motions are widely distributed, emotions focus on the center, indicating the minor changes of facial expressions in most animation samples. Figure \ref{figure:label_motion_vadi}  also shows the distribution of labeled relations w.r.t their dominance and intimacy scores.

\subsection{Animation and interpolation}
\begin{figure}[h]
    \centering
    \includegraphics[width=0.95\linewidth]{images/interpolation_comparison.pdf}
    \caption{The comparison between original rotations and interpolated rotations of the joints: neck, root~(\textit{hips} in Mixamo rigging), left hip~(\textit{left up leg} in Mixamo rigging), and left shoulder for the animation \textit{Quick Informal Bow}.}
    \label{figure:interpolation_comparison}
\end{figure}

\section{VRNN and Transformer-VAE}
Figure \ref{figure:motion_vae_error} compares the performance between Transformer-VAE and VRNN, and the bar plot demonstrates the performance between VRNN and Transformer-VAE for predicting the poses of different body parts.

\begin{figure}[h]
    \centering
    \includegraphics[width=0.95\linewidth]{images/degree_difference.pdf}
    \caption{The comparison between original rotations and predicted rotations of the joints: (a) the density plot of the prediction error from Transformer-VAE; (b) the density plot of the prediction error from VRNN; (c) comparison between Transformer-VAE and VRNN for different body parts. (See detailed classification of joints in the appendix.) }
    \label{figure:motion_vae_error}
\end{figure}

\section{Labels}
Table \ref{table:one} shows label types with label options. %Experimenters need to first label the quality of the animation.
\begin{table}[h]
\centering
  \begin{tabular}{c c c}\toprule
   \textbf{Label}  & \textbf{Option} \\ 
    \midrule
    Quality  & good/medium/bad\\
    \hline
    Dominance score & low/medium/high \\
    Intimacy score & low/medium/high \\
     \bottomrule\\
    % Facial expression name & happy/sad/...  \\
    % \hline
    % Body movement name & jump/bow/...  \\
    % \bottomrule\\
  \end{tabular}
    \caption{Scene labels and options}
     \label{table:one}
\end{table}
